# Supplementary material for: Hiding Local Manipulations on SAR Images: a Counter-Forensic Attack
Source: arXiv:2407.07041 source file (2025-03-14)
Supplement: Supplementary file 1 [file appendix.tex]

\section{Analysis of the Detector Performance on Downscaling Edited Images}
\label{sec:appendix}

As shown in Section~\ref{subsec:results_attack}, Table~\ref{tab:result_attack_nospeckle}, a strong downscaling operation applied to the donor image when creating the splicing is difficult to spot by the state-of-the-art forensic detectors, even in absence of counter-forensic attacks.
This behaviour was not shown in the original detectors' paper~\cite{cannas2022amplitude}. In this appendix, we perform additional experiments to investigate more in depth the issue. 
We start showing more detailed detection results on downscaled images; then, we perform further investigations on \gls{sar} products in the frequency domain.
%; finally, we compare different versions of the \gls{sar} forensic detector trained on resampled images. 

\subsection{Detailed detection results in case of downscaling}
\label{subsec:appendix_detection_downscaling}

At first, we refine the set of possible downscaling factors applied to the donor image with respect to the post-processing parameters shown in Table~\ref{tab:setup_editing}.
Specifically, we generate local image splicing by applying downscaling with factors in the set $\{0.5, 0.525, 0.55, 0.6, 0.65, 0.7, 0.75, 0.8, 0.85, 0.9, 0.95 \}$. The first four factors belong to the ``Downscale Far'' scenario, all the others to the ``Downscale Near'' one. 

The achieved localization results in absence of attack are depicted in Table~\ref{tab:appendix_downscaling_noattack}.
Notice that they are in line with those previously shown in Table~\ref{tab:result_attack_nospeckle}: overall, 
the higher the factor, the better the detection performance. 
This is even more perceivable by looking at Fig.~\ref{fig:appendix_downscaling}, which shows the performance enhancement as dowscaling factors approach the $1$.
%(i.e., stronger downscaling achieves lower performances), 
An exception occurs for the $\times 0.5$ setup, which does not report extremely bad localization results, being comparable with lighter dowscaling.
%Overall, apart from very low downscaling factors, the higher the factor, the better the detection performance. 

Even if these results might seem counterintuitive at a first sight, it is well-known in the image forensics literature that spotting downscaling artifacts is a more challenging task than exposing upscaling traces~\cite{Popescu2005, kirchner2008fast_resampling, kirchner2019cnn_resampling}.
In all these papers, which investigate standard $8$-bit imagery, it is pointed out that downscaling factors in the range $(0.5, 0.8]$ are harder to detect than higher factors. 
Moreover, it is also specified that the $\times 0.5$ situation is a well-known corner case which produces different artifacts than other factors \cite{kirchner2019cnn_resampling, pasquini2018information}.
However, if the $\times 0.5$ scenario usually reports extremely bad performances in state-of-the-art, it is worth noticing that the employed \gls{sar} forensic detectors show good \glspl{auc}, similar to those achieved for the $\times0.7$ case. 

\begin{table*}[t]
\caption{Averae AUC achieved in absence of counter-forensic attack, for different downscaling factors.}
\label{tab:appendix_downscaling_noattack}
\centering
\resizebox{.8\textwidth}{!}{
\begin{tabular}{@{}llccccccccccc@{}}
\toprule
                 & &  \multicolumn{11}{c}{Downscaling Factor}   \\ \cmidrule(l){3-13} 
Detector             &  & \multicolumn{1}{c}{$\times 0.5$}  & \multicolumn{1}{c}{$\times 0.525$} & \multicolumn{1}{c}{$\times 0.55$} & \multicolumn{1}{c}{$\times 0.6$} & \multicolumn{1}{c}{$\times 0.65$} & \multicolumn{1}{c}{$\times 0.7$} & \multicolumn{1}{c}{$\times 0.75$} & \multicolumn{1}{c}{$\times 0.8$} & \multicolumn{1}{c}{$\times 0.85$} & \multicolumn{1}{c}{$\times 0.9$} & \multicolumn{1}{c}{$\times 0.95$}
\\ 
\midrule
SAE    &  &$0.779$ & $0.679$ &$0.673$ & $0.666$  & $0.717$  & $0.763$ & $0.826$ & $0.866$ & $0.887$ & $0.905$ & $0.918$\\
ASAE    & &$0.748$ &$0.653$  & $0.647$  & $0.642$  &$0.712$  & $0.766$ & $0.830$ & $0.877$ & $0.905$ & $0.935$ & $0.957$\\
\bottomrule
\end{tabular}

}
\end{table*}

\begin{figure}[t]
  \centering  
  \includegraphics[width=\columnwidth]{figures/appendix_downscaling_results.pdf}
  \caption{Average AUC achieved in absence of counter-forensic attack, for different downscaling factors. }
  \label{fig:appendix_downscaling}
\end{figure}

\subsection{Frequency domain investigations}
\label{subsec:appendix_frequency}

%To further investigate on the resampling artifacts, w
We perform additional experiments in the frequency domain, considering pristine samples and modified versions of them which underwent different downscaling and upscaling operations.
For each sample, we compute the azimuthal integration of the squared frequency spectrum over radial frequencies $\FA_{\I}(f)$, as defined in \eqref{eq:azimuthal_spectrum}. 
Fig.~\ref{fig:appendix_resampling_singleprod} shows the average $\FA_{\I}(f)$ for downscaled (\ref{fig:appendix_downscaling_singleprod}) and upscaled (\ref{fig:appendix_upscaling_singleprod}) images of a single \gls{sar} product. 
Fig.~\ref{fig:appendix_fft_products} shows the average $\FA_{\I}(f)$ of pristine samples, for all the $24$ different \gls{sar} products considered in this study.

In Fig.~\ref{fig:appendix_upscaling_singleprod}, the upscaling artifacts are clearly visible and follow a specific trend: as the upscaling factor increases, the energy of the spectrum concentrates at lower frequencies. 
The effects of downscaling (see Fig.~\ref{fig:appendix_downscaling_singleprod}) are more variable and depend on the factors used. 
Strong downscaling produces an almost flat spectrum after few frequency samples ($100$ samples, approximately); lighter downscaling leaves less pronounced artifacts. 

If we compare the spectrum of the resampled data with the original ones shown in Fig.~\ref{fig:appendix_fft_products}, we can guess a similarity between pristine spectra and those produced by upscaling and ligth downscaling, meaning that a single product spectrum could be approximately seen as the resized version of another one.
This behaviour is reasonable, if we consider that different products bring distinct resampling artifacts due to the execution process done for generating them \cite{cannas2022amplitude}.

In contrast, none of the pristine spectra shows a flat behaviour versus frequency. 
We conjecture that this characteristic can be one possible reason of performance degradation in case of strong downscaling. 
Indeed, the considered forensic detectors are trained over only pristine samples (\gls{sae}) or over pristine and upscaled version of them (\gls{asae}). It is reasonable to assume that the strong downscaling frequency artifacts follow a completely different pattern than those seen during training, thus being more challenging to detect.
%QUESTO NON SPIEGA LO 0.5 MA SU QUESTO AL MOMENTO NON ABBIAMO IDEA XD

\begin{figure*}[t]
  \centering  
    \begin{subfigure}[b]{\textwidth}
        \centering
          \includegraphics[width=\textwidth]{figures/appendix_downscaling_singleprod.pdf}
          \caption{Downscaling factors. }
          \label{fig:appendix_downscaling_singleprod}
    \end{subfigure}
\hfill
    \begin{subfigure}[b]{\textwidth}
        \centering
        \includegraphics[width=\columnwidth]{figures/appendix_upscaling_singleprod.pdf}
        \caption{Upscaling factors.}
        \label{fig:appendix_upscaling_singleprod}
    \end{subfigure}
  \caption{Azimuthal integration of the squared frequency spectrum over radial frequency samples, considering different resizing factors. Results are averaged over the images of a single SAR product. }
  \label{fig:appendix_resampling_singleprod}
\end{figure*}

\begin{figure}[t]
  \centering  
  \includegraphics[width=\columnwidth]{figures/appendix_fft_products.pdf}
  \caption{Azimuthal integration of the squared frequency spectrum over radial frequency samples. Every line corresponds to the average result across the images of a single SAR product. }
  \label{fig:appendix_fft_products}
\end{figure}
